# Supplementary material for: Quantum-Fisher-information-aware optimization yields a quantum reservoir advantage over tuned classical reservoirs
Source: arXiv:2610.14454 source file (2026-10-10)
Supplement: Supplementary file 2 [file benchmark_macros.tex]

\newcommand{\rGainMin}{24.9}
\newcommand{\rGainMinM}{6}
\newcommand{\rGainMax}{69.4}
\newcommand{\rGainMaxM}{16}
\newcommand{\rShareFloor}{99.5}
\newcommand{\rShareMin}{99.54}
\newcommand{\rShareMinM}{6}
\newcommand{\rShareOthers}{; $99.97\%$ at $m=8$ and $99.93\%$ at $m=30$; $100.0\%$ otherwise}
\newcommand{\rBoAheadRange}{21--50}
\newcommand{\rBoAheadMs}{$m\le24$}
\newcommand{\rBoBehind}{behind it by $34\%$ at $m=30$ (only $3.0\%$ of the draws are worse)}
\newcommand{\rStageSmall}{1.2, 3.4 and 5.7\%}
\newcommand{\rStageSmallMs}{$4$, $6$ and $8$}
\newcommand{\rStageLargeRange}{29--51}
\newcommand{\rStageLargeList}{$29.1\%$ at $m=12$, $39.2\%$ at $m=16$, $44.3\%$ at $m=18$, $38.1\%$ at $m=24$ and $51.4\%$ at $m=30$}
\newcommand{\rTrainLossSmall}{2--11}
\newcommand{\rTrainLossLarge}{56--76}
\newcommand{\rBoGainA}{21.2}
\newcommand{\rQfiGainA}{51.3}
\newcommand{\rBoGainB}{33.6}
\newcommand{\rQfiGainB}{35.1}
\newcommand{\rAltGains}{$+53.4\%$ and $+50.5\%$}
\newcommand{\rAltStage}{$40.6\%$ and $31.3\%$}
\newcommand{\rPhiMove}{1--26}
\newcommand{\rBoEvals}{114--343}
\newcommand{\rNcRest}{$1.6\times10^{-3}$}
\newcommand{\rNcWorst}{$8.1\times10^{-2}$}
\newcommand{\rNcWorstM}{16}
\newcommand{\rNcPending}{all closing tasks are complete}
\newcommand{\rShotFour}{0.36--0.71}
\newcommand{\rShotFive}{0.23--0.58}
\newcommand{\rShotSix}{0.17--0.40}
\newcommand{\rNstarRefitMin}{6.6\times10^{6}}
\newcommand{\rNstarRefitMinM}{16}
\newcommand{\rNstarRefitMax}{2.1\times10^{10}}
\newcommand{\rNstarRefitMaxM}{8}
\newcommand{\rNstarFixedMin}{1.1\times10^{7}}
\newcommand{\rNstarFixedMax}{7.6\times10^{11}}
\newcommand{\rNstarDecades}{10^{6}$--$10^{11}}
\newcommand{\rShotAbove}{above the ESN mean at every $m$}
\newcommand{\rPhoton}{The photon cap is active at $m=4$ and $m=6$ ($\max_t\langle n\rangle=3.000$)}
\newcommand{\rFaces}{; the end point at $m=8$ sits on the widened face of $\gamma_1$, where the widening rule stopped because the arm had converged; no end point sits on the $|\tilde u_t|$ cap.}
\newcommand{\rBudgetList}{$12$ (two atoms), $12$ (one atom), $16$ (three atoms), $16$ (one atom), $18$ and $24$}
\newcommand{\rInterimSentence}{Every QFI stage had finished when the tables were built.}
\newcommand{\rInterimCaveat}{}
\newcommand{\rBuildStamp}{2026-10-09 16:32 MST}
\newcommand{\rDimMin}{11}
\newcommand{\rDimMax}{44}
\newcommand{\rDimList}{$m=4$: 11; $m=6$: 16; $m=8$: 16; $m=12$: 23/21; $m=16$: 30/26; $m=18$: 30; $m=24$: 37; $m=30$: 44}
\newcommand{\rEsnNSettings}{810}
\newcommand{\rEsnNSettingsOrig}{300}
\newcommand{\rEsnLevelsRadius}{\{0.1, 0.2, 0.3, 0.5, 0.7, 0.9, 0.95, 0.99, 1.1\}}
\newcommand{\rEsnLevelsLeak}{\{0.1, 0.3, 0.5, 0.7, 1.0\}}
\newcommand{\rEsnLevelsScale}{\{0.005, 0.01, 0.02, 0.05, 0.1, 0.3, 0.5, 1.0, 2.0\}}
\newcommand{\rEsnLevelsBias}{\{0, 1\}}
\newcommand{\rEsnRepro}{0}
\newcommand{\rEsnSettingsList}{$m=4$: $(0.7, 1.0, 0.02, 0)$ (leak $=1.0$ (grid maximum)); $m=6$: $(0.9, 1.0, 0.02, 0)$ (leak $=1.0$ (grid maximum)); $m=8$: $(0.9, 1.0, 0.05, 0)$ (leak $=1.0$ (grid maximum)); $m=12$: $(0.9, 1.0, 0.05, 0)$ (leak $=1.0$ (grid maximum)); $m=16$: $(0.2, 0.1, 1.0, 0)$ (leak $=0.1$ (grid minimum)); $m=18$: $(0.2, 0.1, 1.0, 0)$ (leak $=0.1$ (grid minimum)); $m=24$: $(0.3, 0.1, 1.0, 1)$ (leak $=0.1$ (grid minimum)); $m=30$: $(0.7, 0.3, 0.5, 0)$}
\newcommand{\rEsnLeakMaxMs}{$4$, $6$, $8$ and $12$}
\newcommand{\rEsnLeakMinMs}{$16$, $18$ and $24$}
\newcommand{\rExtTopSpreadMin}{0.009}
\newcommand{\rExtTopSpreadMax}{0.013}
\newcommand{\rCtrlRatioBestList}{$m=4$: 1.024; $m=6$: 1.026; $m=8$: 1.117; $m=12$: 0.867; $m=16$: 0.825; $m=18$: 0.797; $m=24$: 0.977; $m=30$: 0.980}
\newcommand{\rCtrlRatioZList}{1.014 ($m=4$), 0.989 ($m=6$), 0.976 ($m=8$), 0.856 ($m=12$), 0.751 ($m=16$), 0.669 ($m=18$), 0.977 ($m=24$) and 0.980 ($m=30$)}
\newcommand{\rCtrlRatioBOList}{1.024 ($m=4$), 1.026 ($m=6$), 1.117 ($m=8$), 0.867 ($m=12$), 0.825 ($m=16$), 0.797 ($m=18$), 0.945 ($m=24$) and 0.952 ($m=30$)}
\newcommand{\rCtrlRatioThetaList}{1.000 ($m=4$), 0.998 ($m=6$), 0.944 ($m=8$), 0.769 ($m=12$), 0.693 ($m=16$), 0.800 ($m=18$), 0.953 ($m=24$) and 0.952 ($m=30$)}
\newcommand{\rCtrlBelowMid}{$13\%$ at $m=12$, $17\%$ at $m=16$ and $20\%$ at $m=18$}
\newcommand{\rCtrlBelowMidRange}{13--20}
\newcommand{\rCtrlBestMid}{BO$_{\rm eq}$ at $m=$ $12$, $16$ and $18$}
\newcommand{\rCtrlAboveSmall}{$2\%$ at $m=4$, $3\%$ at $m=6$ and $12\%$ at $m=8$}
\newcommand{\rCtrlAboveSmallRange}{2--12}
\newcommand{\rCtrlBestSmall}{BO$_{\rm eq}$ at $m=$ $4$, $6$ and $8$}
\newcommand{\rCtrlZGainA}{2.5}
\newcommand{\rCtrlThetaGainA}{1.2}
\newcommand{\rCtrlBOeqGainA}{3.4}
\newcommand{\rCtrlCGainA}{1.2}
\newcommand{\rCtrlZGainB}{2.4}
\newcommand{\rCtrlThetaGainB}{3.2}
\newcommand{\rCtrlBOeqGainB}{5.9}
\newcommand{\rCtrlCGainB}{3.4}
\newcommand{\rCtrlZGainC}{3.4}
\newcommand{\rCtrlThetaGainC}{0.0}
\newcommand{\rCtrlBOeqGainC}{15.5}
\newcommand{\rCtrlCGainC}{5.7}
\newcommand{\rCtrlZGainD}{17.2}
\newcommand{\rCtrlThetaGainD}{7.9}
\newcommand{\rCtrlBOeqGainD}{18.2}
\newcommand{\rCtrlCGainD}{29.1}
\newcommand{\rCtrlZGainE}{19.0}
\newcommand{\rCtrlThetaGainE}{12.3}
\newcommand{\rCtrlBOeqGainE}{26.3}
\newcommand{\rCtrlCGainE}{39.2}
\newcommand{\rCtrlZGainF}{16.8}
\newcommand{\rCtrlThetaGainF}{30.5}
\newcommand{\rCtrlBOeqGainF}{30.2}
\newcommand{\rCtrlCGainF}{44.3}
\newcommand{\rCtrlZGainG}{3.3}
\newcommand{\rCtrlThetaGainG}{0.8}
\newcommand{\rCtrlBOeqGainG}{0.0}
\newcommand{\rCtrlCGainG}{5.5}
\newcommand{\rCtrlZGainH}{2.8}
\newcommand{\rCtrlThetaGainH}{0.0}
\newcommand{\rCtrlBOeqGainH}{0.0}
\newcommand{\rCtrlCGainH}{4.8}
\newcommand{\rCtrlGainsMid}{$m=12$: 17.2 / 7.9 / 18.2 / 29.1\%; $m=16$: 19.0 / 12.3 / 26.3 / 39.2\%; $m=18$: 16.8 / 30.5 / 30.2 / 44.3\%}
\newcommand{\rCtrlGainsSmall}{$m=4$: 2.5 / 1.2 / 3.4 / 1.2\%; $m=6$: 2.4 / 3.2 / 5.9 / 3.4\%; $m=8$: 3.4 / 0.0 / 15.5 / 5.7\%}
\newcommand{\rCtrlGainsLargeBlockOne}{$m=24$: 3.3 / 0.8 / 0.0 / 5.5\%; $m=30$: 2.8 / 0.0 / 0.0 / 4.8\%}
\newcommand{\rThetaRecoveryMid}{$27\%$ ($m=12$), $31\%$ ($m=16$) and $69\%$ ($m=18$)}
\newcommand{\rThetaRecoveryMidRange}{27--69}
\newcommand{\rSeqQngShares}{$94\%$ ($m=4$), $89\%$ ($m=6$), $23\%$ ($m=8$), $34\%$ ($m=12$), $44\%$ ($m=16$), $47\%$ ($m=18$), $10\%$ ($m=24$) and $30\%$ ($m=30$)}
\newcommand{\rSeqQngShareMidRange}{34--47}
\newcommand{\rSeqQngShareSmallAB}{94\% and 89\%}
\newcommand{\rPrevZpHeldA}{0.0417}
\newcommand{\rPrevQfiHeldA}{0.0416}
\newcommand{\rPrevBOHeldA}{0.0599}
\newcommand{\rPrevStartHeldA}{0.0636}
\newcommand{\rPrevRatioQfiZpA}{1.000}
\newcommand{\rPrevRatioQfiBOA}{0.696}
\newcommand{\rPrevRatioCBestA}{0.945}
\newcommand{\rPrevCBelowA}{6}
\newcommand{\rPrevZpGainA}{34.5}
\newcommand{\rPrevBOGainA}{5.9}
\newcommand{\rPrevQfiGainA}{34.6}
\newcommand{\rPrevCGainA}{38.1}
\newcommand{\rPrevZpLossA}{0.09376}
\newcommand{\rPrevQfiLossA}{0.08925}
\newcommand{\rBlockOneRatioBestA}{0.977}
\newcommand{\rBlockOneCLossGainA}{13}
\newcommand{\rPrevZpHeldB}{0.0766}
\newcommand{\rPrevQfiHeldB}{0.0417}
\newcommand{\rPrevBOHeldB}{0.0717}
\newcommand{\rPrevStartHeldB}{0.0816}
\newcommand{\rPrevRatioQfiZpB}{0.544}
\newcommand{\rPrevRatioQfiBOB}{0.581}
\newcommand{\rPrevRatioCBestB}{0.553}
\newcommand{\rPrevCBelowB}{45}
\newcommand{\rPrevZpGainB}{6.2}
\newcommand{\rPrevBOGainB}{12.2}
\newcommand{\rPrevQfiGainB}{49.0}
\newcommand{\rPrevCGainB}{51.4}
\newcommand{\rPrevZpLossB}{0.29410}
\newcommand{\rPrevQfiLossB}{0.09258}
\newcommand{\rBlockOneRatioBestB}{0.980}
\newcommand{\rBlockOneCLossGainB}{14}
\newcommand{\rMidCLossGainRange}{56--70}
\newcommand{\rCtrlPhotonMs}{$4$ and $6$}
\newcommand{\rCtrlPhotonBO}{1.535 and 2.652}
\newcommand{\rCtrlThetaBudgetMs}{$12$, $16$ and $18$}
\newcommand{\rCtrlZBudgetMs}{none}
\newcommand{\rCtrlEvalsC}{371--3,255}
\newcommand{\rCtrlEvalsZ}{138--709}
\newcommand{\rCtrlEvalsTheta}{209--3,828}
\newcommand{\rExtEsnChanges}{$-16\%$ ($m=4$), $-5\%$ ($m=6$), $-3\%$ ($m=8$), $-1\%$ ($m=12$), $-6\%$ ($m=16$) and $-8\%$ ($m=18$)}
\newcommand{\rExtEsnUnchangedMs}{$24$ and $30$}
\newcommand{\rExtGainRange}{25--69}
\newcommand{\rOrigGainRange}{29--71}
\newcommand{\rExtShareFloor}{99.5}
\newcommand{\rOrigShareFloor}{99.9}
\newcommand{\rExtMinBelowMs}{$m=6$ (0.1416), $m=8$ (0.1192) and $m=30$ (0.0364)}
\newcommand{\rExtRankOrig}{32 ($m=4$), 11 ($m=6$), 6 ($m=8$), 2 ($m=12$), 2 ($m=16$), 4 ($m=18$), 1 ($m=24$) and 1 ($m=30$)}
\newcommand{\rRidgeQrcTen}{6 of 8}
\newcommand{\rRidgeQrcOther}{$10^{-8}$ at $m=4$ and $10^{-6}$ at $m=6$}
\newcommand{\rRidgeEsnShare}{96--100}
\newcommand{\rRidgeMaxChange}{$1.6\times10^{-4}$}
\newcommand{\rSelBeat}{$m=6$ ($-14.2\%$) and $m=8$ ($-6.4\%$)}
\newcommand{\rSelTie}{$m=30$ ($-5.5\%$, interval $[-26\%, +10\%]$)}
\newcommand{\rSelLose}{$m=4$ ($+5.4\%$), $m=12$ ($+38.9\%$), $m=16$ ($+48.2\%$), $m=18$ ($+34.0\%$) and $m=24$ ($+17.0\%$)}
\newcommand{\rSelOrig}{$m=4$: $-1.7\%$, $m=6$: $+7.6\%$, $m=8$: $+10.9\%$, $m=12$: $+33.7\%$, $m=16$: $+45.1\%$, $m=18$: $+27.1\%$, $m=24$: $+22.4\%$ and $m=30$: $-5.5\%$}
\newcommand{\rSelRankRange}{1--6}
\newcommand{\rSelRRange}{0.95--0.99}
\newcommand{\rBsHalfWidth}{10--17}
\newcommand{\rBsStageSmall}{$1.2\%$ $[1.1, 1.2]$ at $m=4$, $3.4\%$ $[2.9, 3.9]$ at $m=6$ and $5.7\%$ $[4.4, 6.6]$ at $m=8$}
\newcommand{\rBsStageMid}{$[24\%, 33\%]$ at $m=12$, $[34\%, 44\%]$ at $m=16$ and $[41\%, 47\%]$ at $m=18$}
\newcommand{\rBsStageLarge}{$[2.8\%, 8.6\%]$ at $m=24$ and $[1.4\%, 8.0\%]$ at $m=30$}
\newcommand{\rBsSharePos}{$100\%$ of the resamples at $m\le24$ and $99.7\%$ at $m=30$}
\newcommand{\rBsMarginMinM}{6}
\newcommand{\rBsMarginMin}{[22\%, 27\%]}
\newcommand{\rBsMarginMaxM}{16}
\newcommand{\rBsMarginMax}{[66\%, 72\%]}
\newcommand{\rFreshQrcRange}{$-7\%$ to $+1\%$}
\newcommand{\rFreshQrcSd}{0.5--2.3}
\newcommand{\rFreshEsnMove}{9}
\newcommand{\rFreshMargins}{$32\%$, $26\%$, $34\%$, $63\%$, $70\%$, $60\%$, $49\%$ and $33\%$}
\newcommand{\rFreshMarginRange}{26--70}
\newcommand{\rFreshStageSmall}{$1.2\%$, $3.4\%$ and $5.7\%$}
\newcommand{\rFreshStageMid}{$30\%$, $41\%$ and $45\%$}
\newcommand{\rFreshStageLarge}{$5.8\%$ and $5.2\%$}
\newcommand{\rFreshExcluded}{at $m=4$ (windows 3, 4) and $m=6$ (windows 3, 4)}
\newcommand{\rFreshMaxnRange}{3.2--4.0}
\newcommand{\rFreshKZeroWorst}{every $m$}
\newcommand{\rSecNcfg}{five}
\newcommand{\rSecMmin}{12}
\newcommand{\rSecPoints}{13,872--18,698}
\newcommand{\rSecRatioBo}{1.2--1.8}
\newcommand{\rSecRatioQfi}{3.1--5.1}
